# Supplementary material for: Quarkonium as relativistic bound state on the light front
Source: arXiv:1704.06968 ancillary file (2017-07-26)
Supplement: Supplementary file 1 [file charmonium.pdf]

$\eta_c(1S)$ 
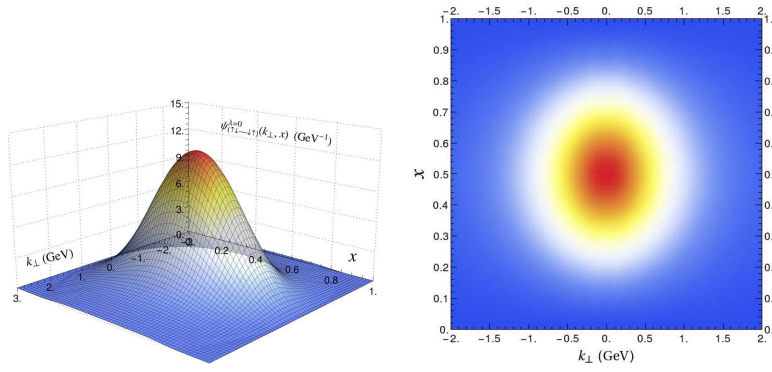

(a)  $\psi_{\uparrow\downarrow-\downarrow\uparrow}^{\lambda=0}(\vec{k}_{\perp}, x)$

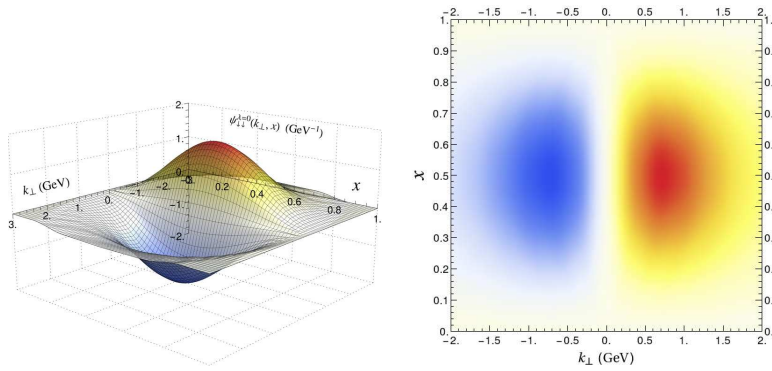

(b)  $\psi_{\downarrow\downarrow}^{\lambda=0}(\vec{k}_{\perp}, x)$

Charmonium: I.  $\eta_c(1S)$

$\eta_c(2S)$ 
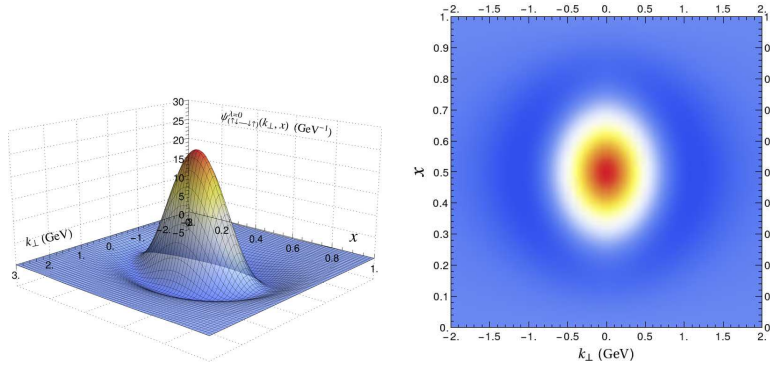

(a)  $\psi_{\uparrow\downarrow-\downarrow\uparrow}^{\lambda=0}(\vec{k}_{\perp}, x)$

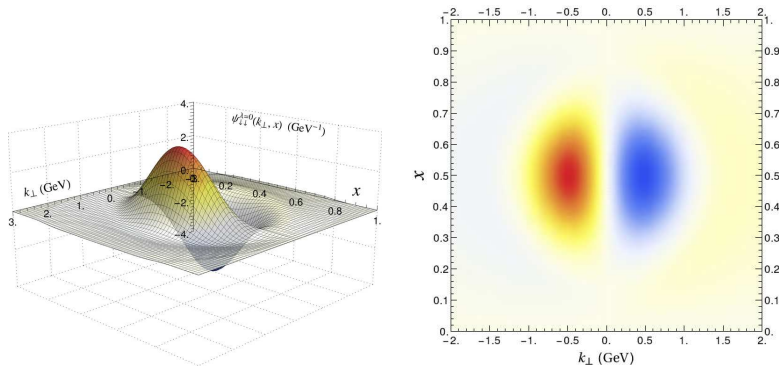

(b)  $\psi_{\uparrow\downarrow}^{\lambda=1}(\vec{k}_{\perp}, x)$

Charmonium: II.  $\eta_c(2S)$

$\eta_c(3S)$ 
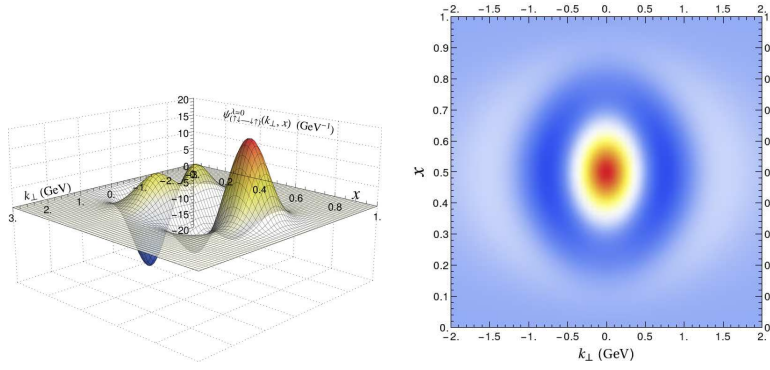

(a)  $\psi_{\uparrow\downarrow \rightarrow \uparrow\uparrow}^{\lambda=0}(\vec{k}_{\perp}, x)$

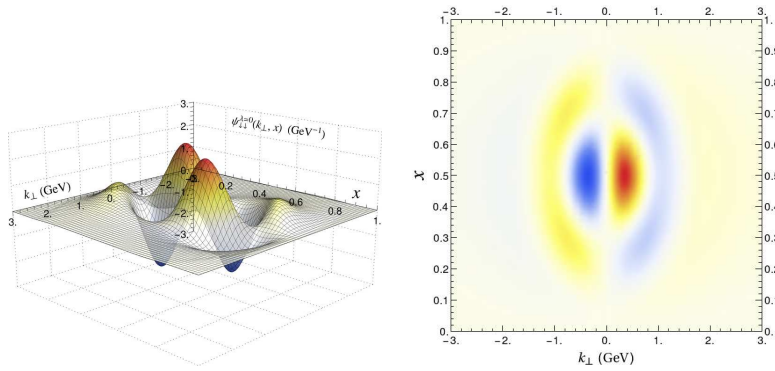

(b)  $\psi_{\uparrow\downarrow}^{\lambda=0}(\vec{k}_{\perp}, x)$

Charmonium: III.  $\eta_c(3S)$

$\chi_{c0}(1P)$ 
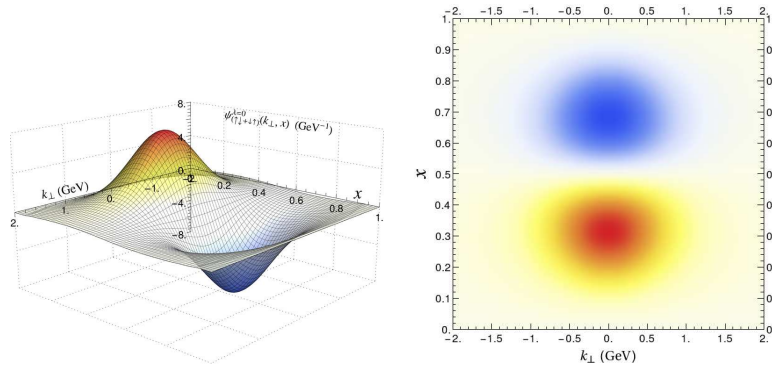

(a)  $\psi_{\uparrow\downarrow+\downarrow\uparrow}^{\lambda=0}(\vec{k}_\perp, x)$

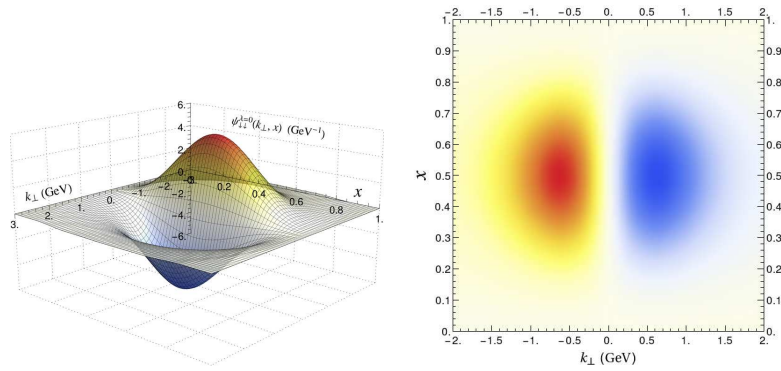

(b)  $\psi_{\downarrow\downarrow}^{\lambda=0}(\vec{k}_\perp, x)$

Charmonium: IV.  $\chi_{c0}(1P)$

$J/\psi$

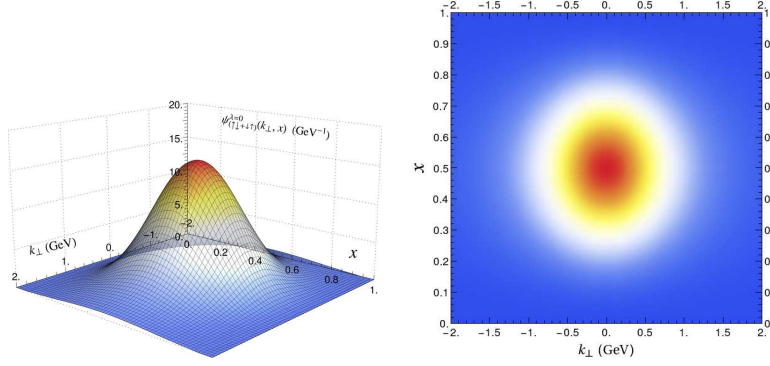

(a)  $\psi_{\uparrow\downarrow+\downarrow\uparrow}^{\lambda=0}(\vec{k}_{\perp}, x)$

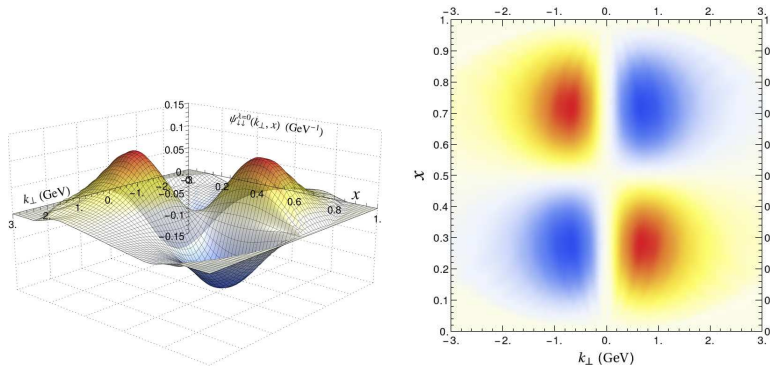

(b)  $\psi_{\uparrow\downarrow}^{\lambda=0}(\vec{k}_{\perp}, x)$

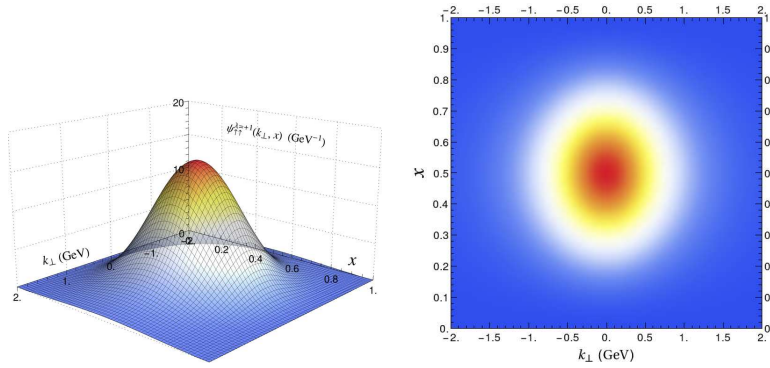

(c)  $\psi_{\uparrow\uparrow}^{\lambda=+1}(\vec{k}_{\perp}, x)$

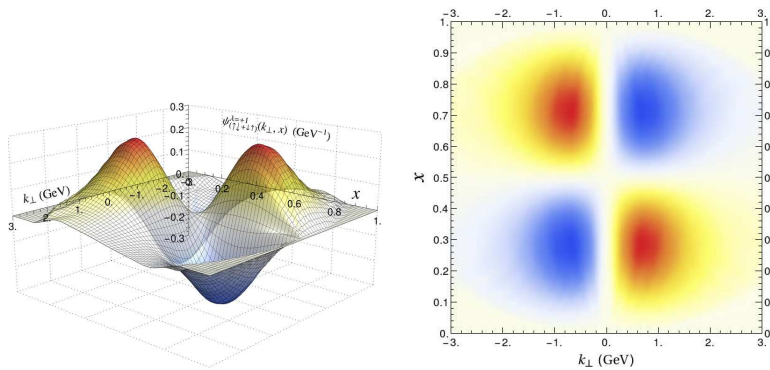

(d)  $\psi_{\uparrow\downarrow+\downarrow\uparrow}^{\lambda=+1}(\vec{k}_{\perp}, x)$

Charmonium: V.  $J/\psi$

$J/\psi$  continued

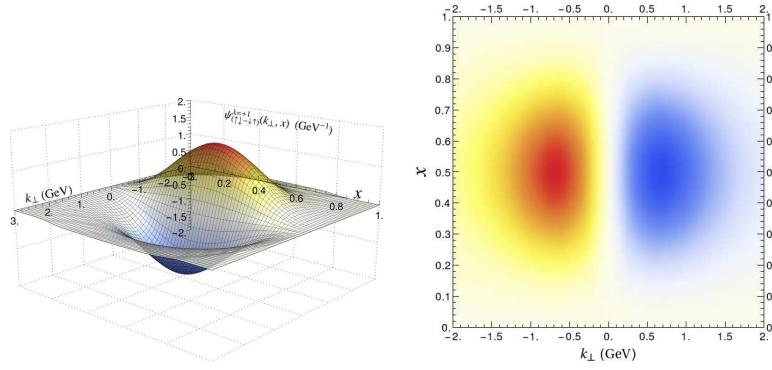

(e)  $\psi_{\uparrow\downarrow}^{\lambda=+1}(\vec{k}_{\perp}, x)$

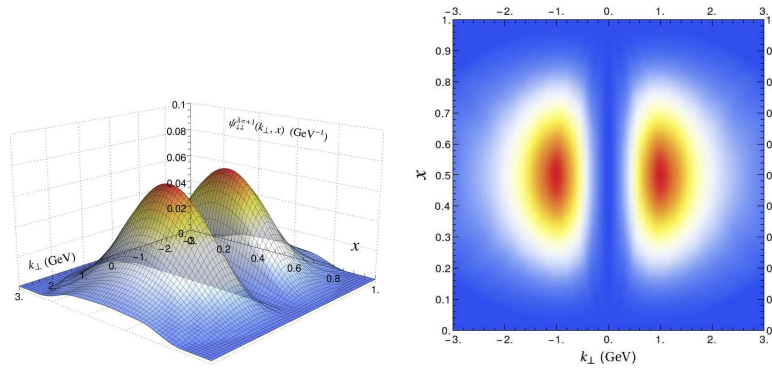

(f)  $\psi_{\downarrow\downarrow}^{\lambda=+1}(\vec{k}_{\perp}, x)$

Charmonium: V.  $J/\psi$



$\psi(2S)$ 
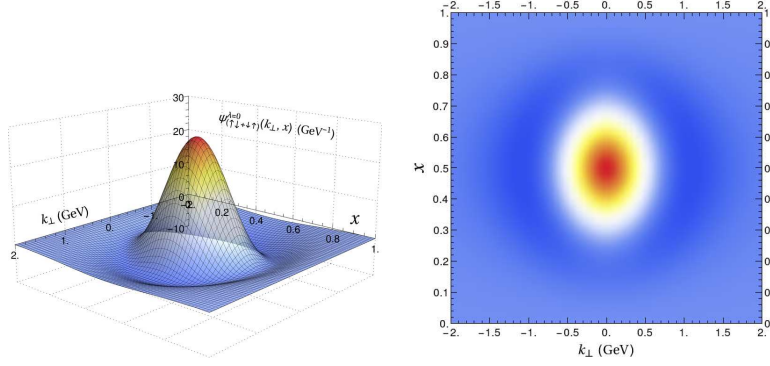

(a)  $\psi_{\uparrow\downarrow\uparrow\downarrow}^{\lambda=0}(\vec{k}_{\perp}, x)$

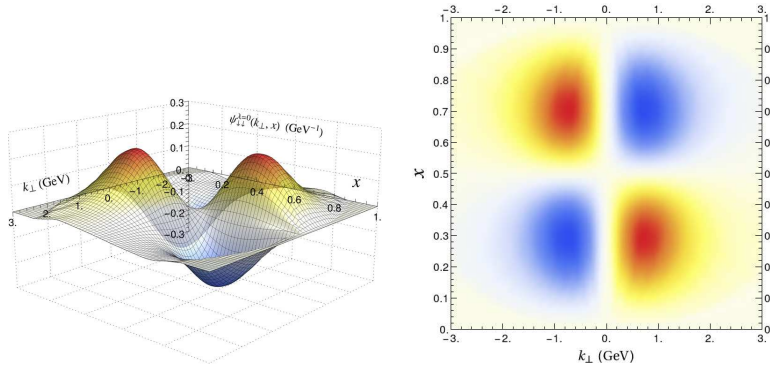

(b)  $\psi_{\downarrow\downarrow}^{\lambda=0}(\vec{k}_{\perp}, x)$

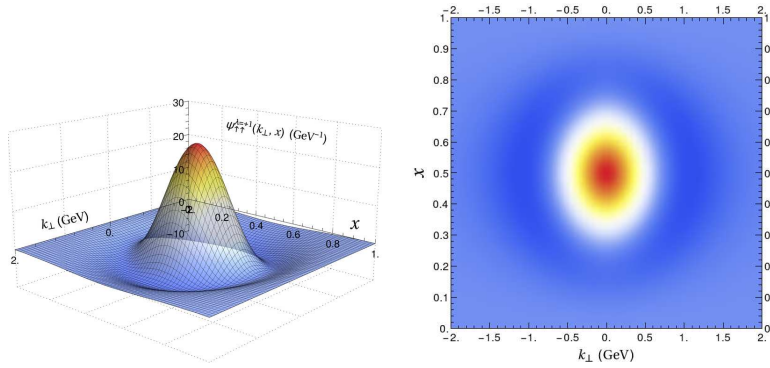

(c)  $\psi_{\uparrow\uparrow}^{\lambda=+1}(\vec{k}_{\perp}, x)$

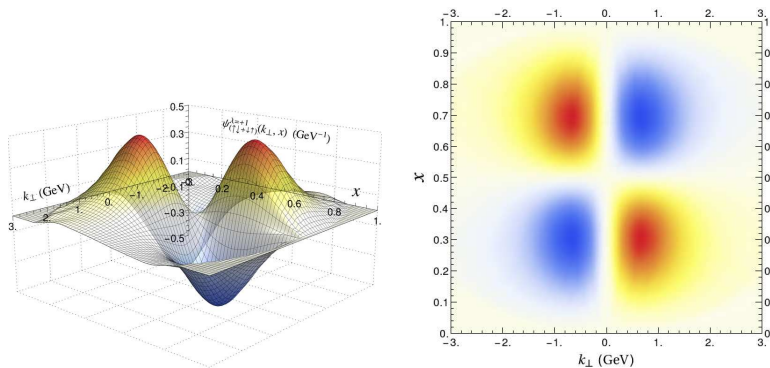

(d)  $\psi_{\downarrow\downarrow\uparrow\uparrow}^{\lambda=+1}(\vec{k}_{\perp}, x)$

Charmonium: VI.  $\psi(2S)$

$\psi(2S)$  continued

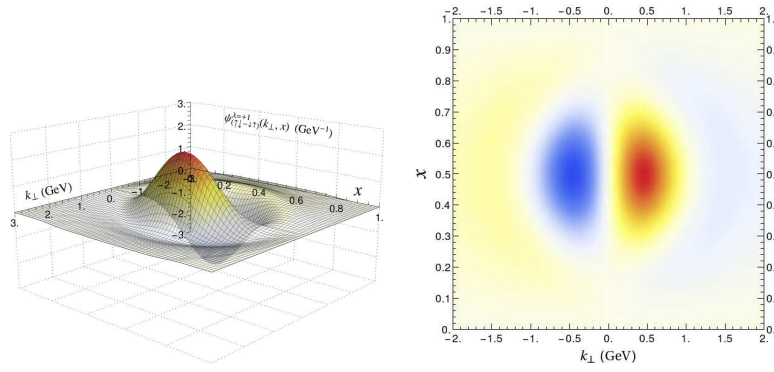

(e)  $\psi_{\uparrow\downarrow-\downarrow\uparrow}^{\lambda=+1}(\vec{k}_{\perp}, x)$

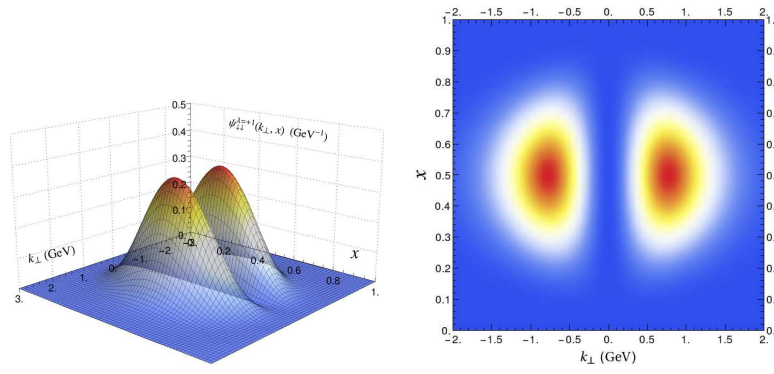

(f)  $\psi_{\downarrow\downarrow}^{\lambda=+1}(\vec{k}_{\perp}, x)$

Charmonium: VI.  $\psi(2S)$



$\psi(3S)$ 
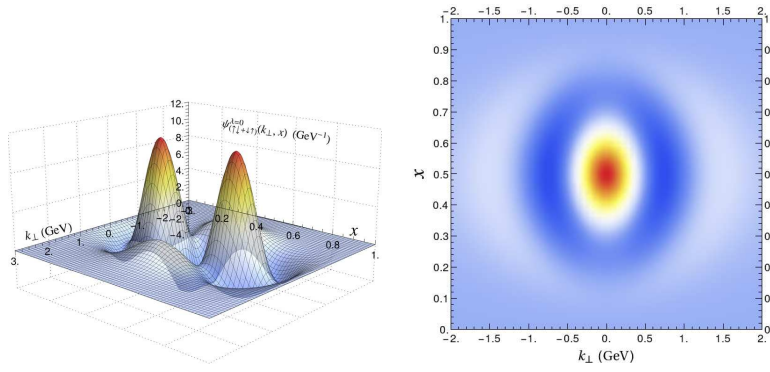

(a)  $\psi_{\uparrow\downarrow+\downarrow\uparrow}^{\lambda=0}(\vec{k}_\perp, x)$

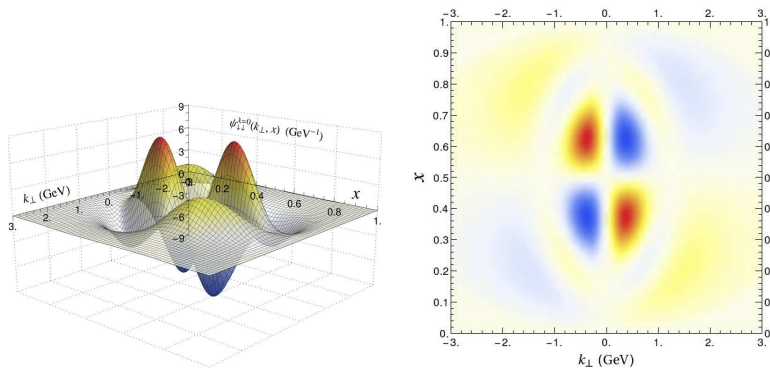

(b)  $\psi_{\uparrow\downarrow}^{\lambda=0}(\vec{k}_\perp, x)$

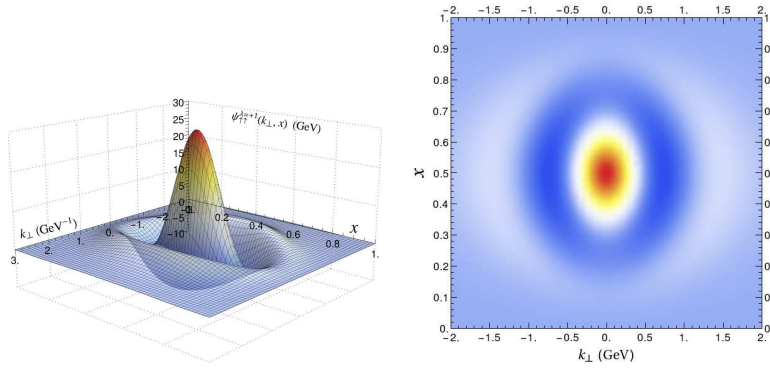

(c)  $\psi_{\uparrow\uparrow}^{\lambda=+1}(\vec{k}_\perp, x)$

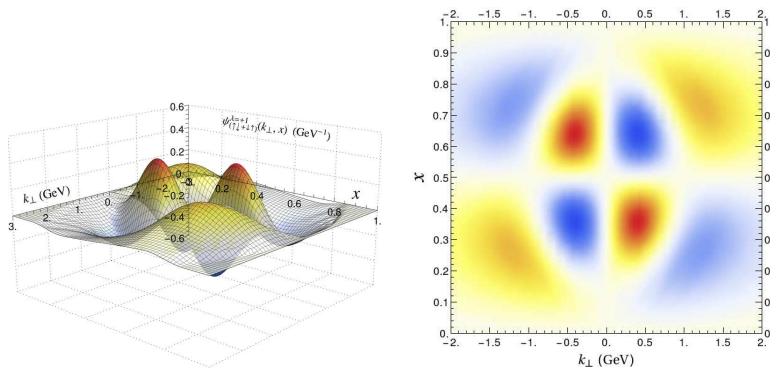

(d)  $\psi_{\uparrow\downarrow+\downarrow\uparrow}^{\lambda=+1}(\vec{k}_\perp, x)$

Charmonium: VII.  $\psi(3S)$

$\psi(3S)$  continued

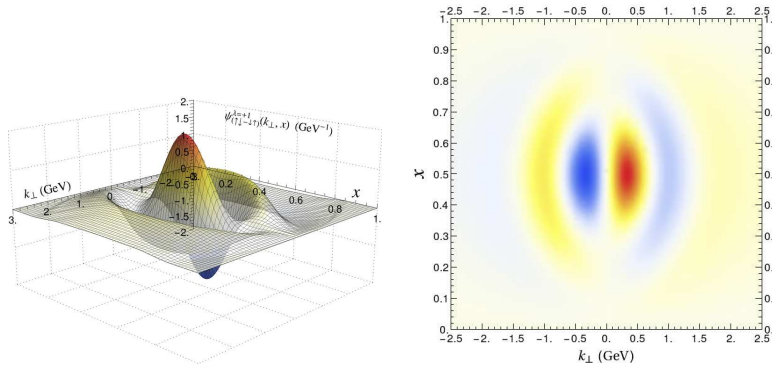

(e)  $\psi_{\uparrow\downarrow-\downarrow\uparrow}^{\lambda=+1}(\vec{k}_{\perp}, x)$

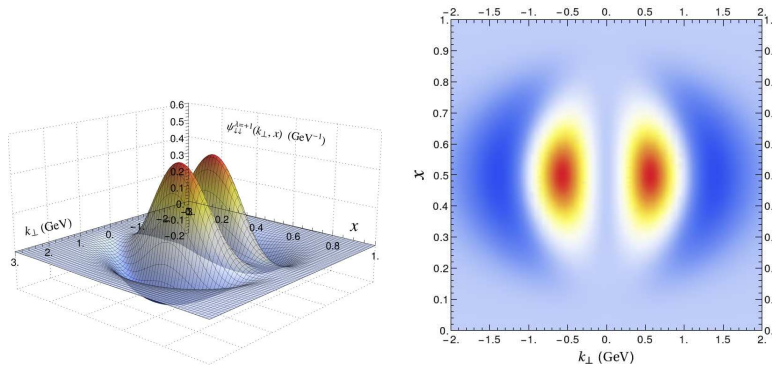

(f)  $\psi_{\downarrow\downarrow}^{\lambda=+1}(\vec{k}_{\perp}, x)$

Charmonium: VII.  $\psi(3S)$

$\psi(1D)$ 
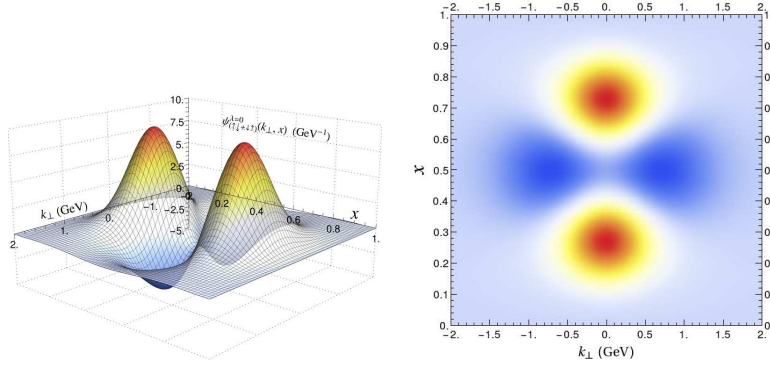

(a)  $\psi_{\uparrow\downarrow+\downarrow\uparrow}^{\lambda=0}(\vec{k}_{\perp}, x)$

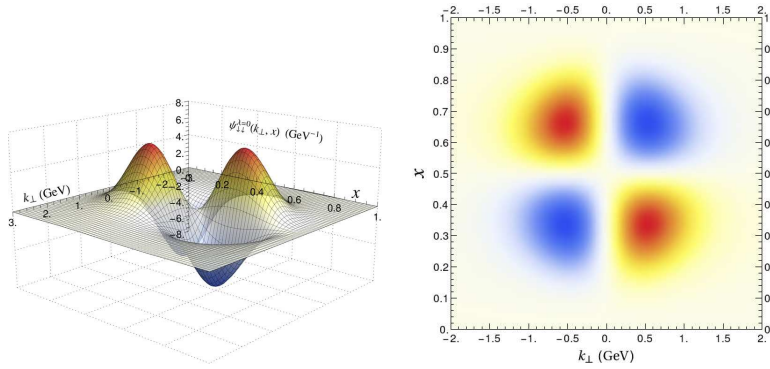

(b)  $\psi_{\uparrow\downarrow}^{\lambda=0}(\vec{k}_{\perp}, x)$

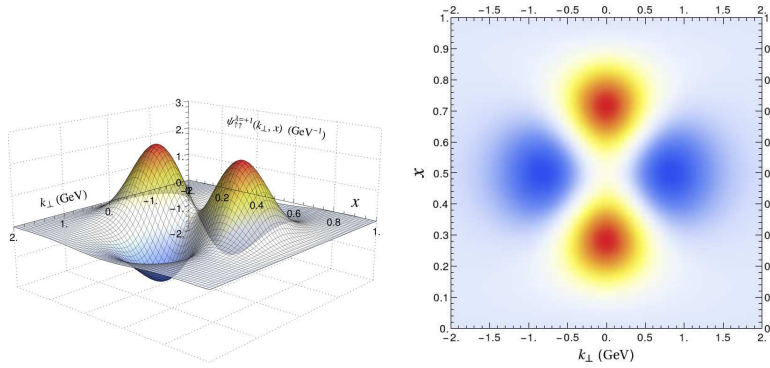

(c)  $\psi_{\uparrow\uparrow}^{\lambda=+1}(\vec{k}_{\perp}, x)$

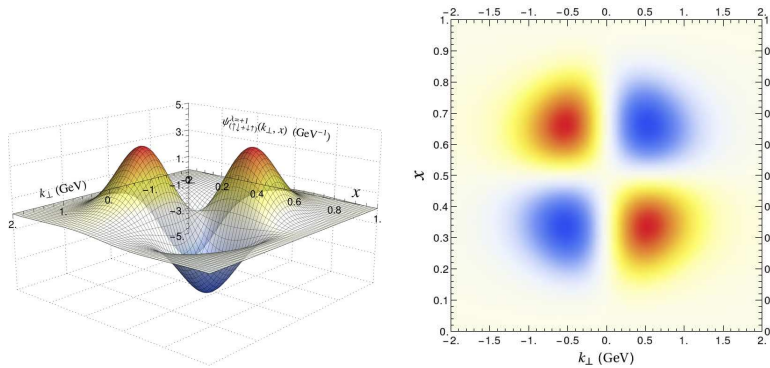

(d)  $\psi_{\uparrow\downarrow+\downarrow\uparrow}^{\lambda=+1}(\vec{k}_{\perp}, x)$

Charmonium: VIII.  $\psi(1D)$

$\psi(1D)$  continued

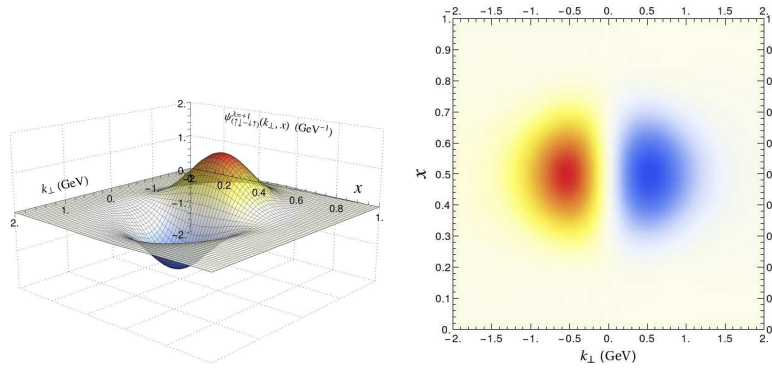

(e)  $\psi_{\uparrow\downarrow-\downarrow\uparrow}^{\lambda=+1}(\vec{k}_{\perp}, x)$

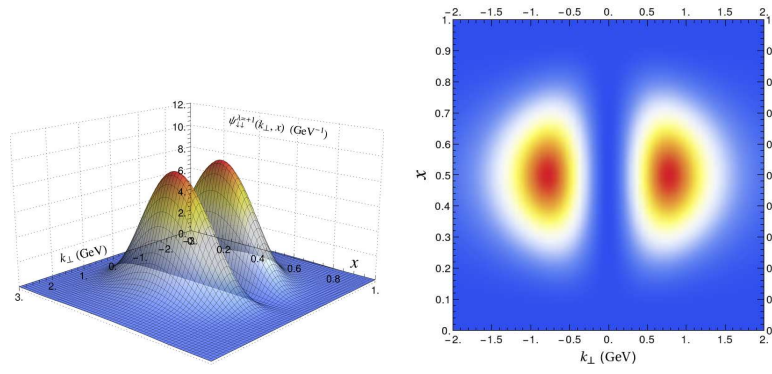

(f)  $\psi_{\downarrow\downarrow}^{\lambda=+1}(\vec{k}_{\perp}, x)$

Charmonium: VIII.  $\psi(1D)$

$\chi_{c1}(1P)$ 
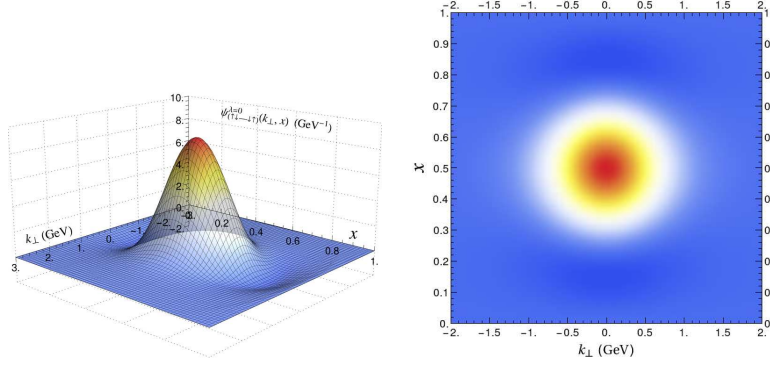

(a)  $\psi_{\uparrow\downarrow-\downarrow\uparrow}^{\lambda=0}(\vec{k}_{\perp}, x)$

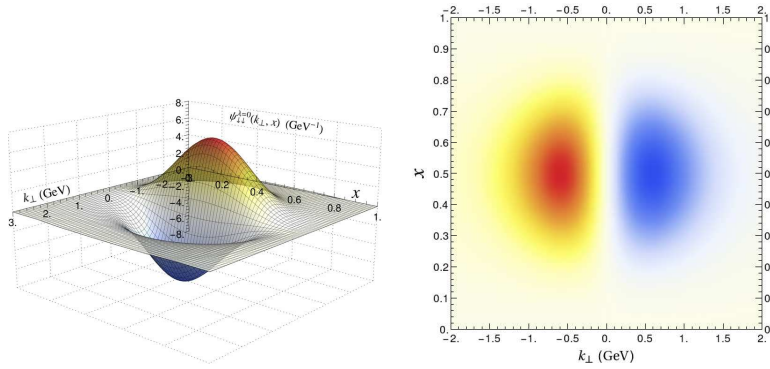

(b)  $\psi_{\uparrow\downarrow}^{\lambda=0}(\vec{k}_{\perp}, x)$

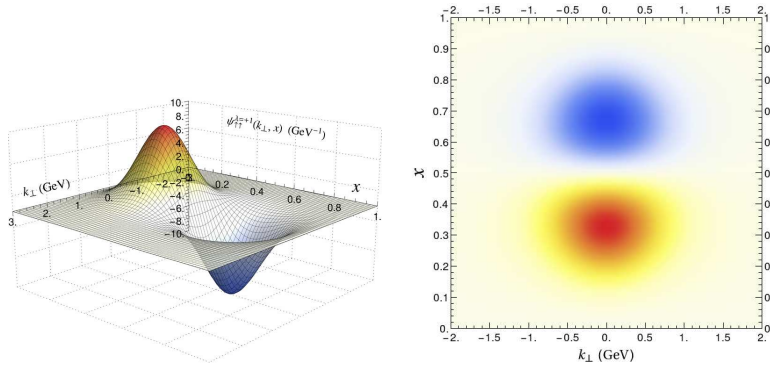

(c)  $\psi_{\uparrow\uparrow}^{\lambda=+1}(\vec{k}_{\perp}, x)$

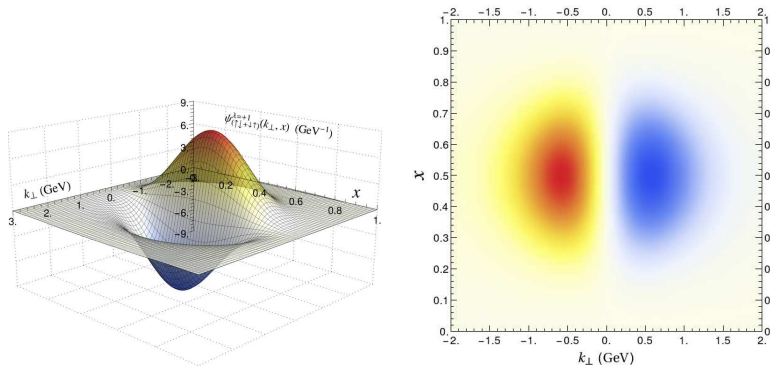

(d)  $\psi_{\uparrow\downarrow+\downarrow\uparrow}^{\lambda=+1}(\vec{k}_{\perp}, x)$

Charmonium: IX.  $\chi_{c1}(1P)$

$\chi_{c1}(1P)$  continued

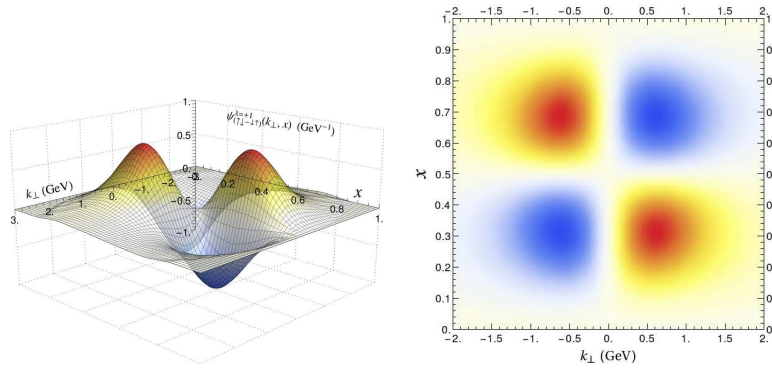

(e)  $\psi_{\uparrow\downarrow-\downarrow\uparrow}^{\lambda=+1}(\vec{k}_\perp, x)$

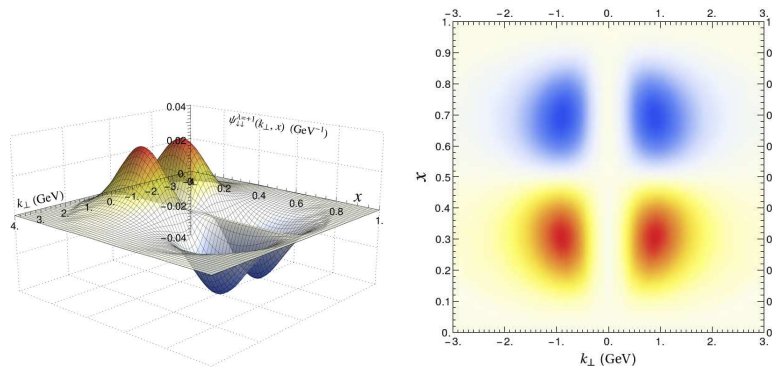

(f)  $\psi_{\uparrow\downarrow}^{\lambda=0}(\vec{k}_\perp, x)$

Charmonium: IX.  $\chi_{c1}(1P)$



$$h_c(1P)$$
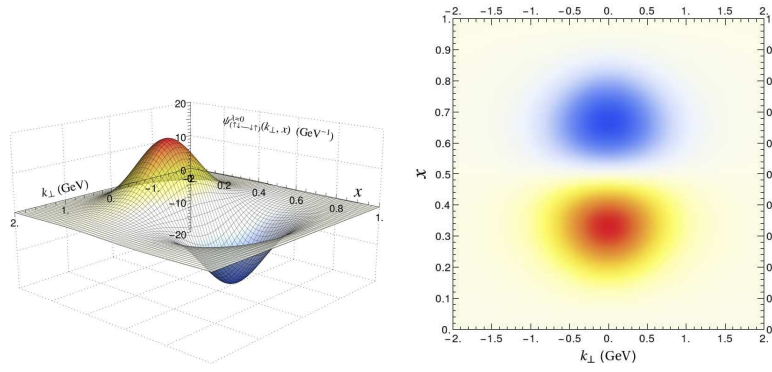

(a)  $\psi_{\uparrow\downarrow\downarrow\uparrow}^{\lambda=0}(\vec{k}_{\perp}, x)$

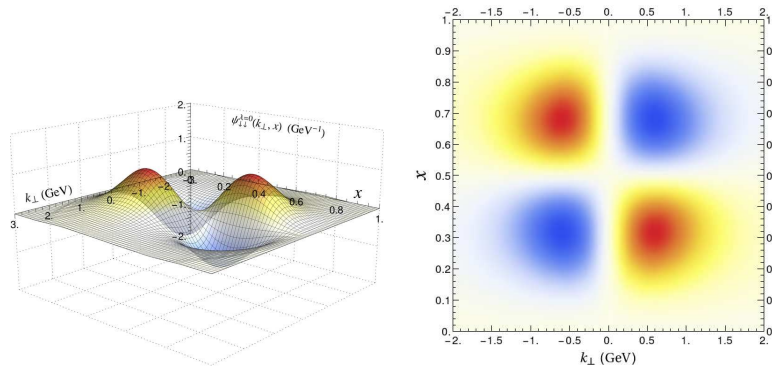

(b)  $\psi_{\uparrow\downarrow}^{\lambda=0}(\vec{k}_{\perp}, x)$

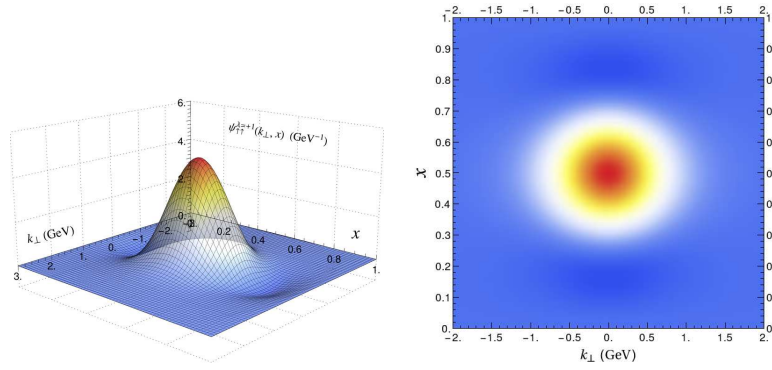

(c)  $\psi_{\uparrow\uparrow}^{\lambda=+1}(\vec{k}_{\perp}, x)$

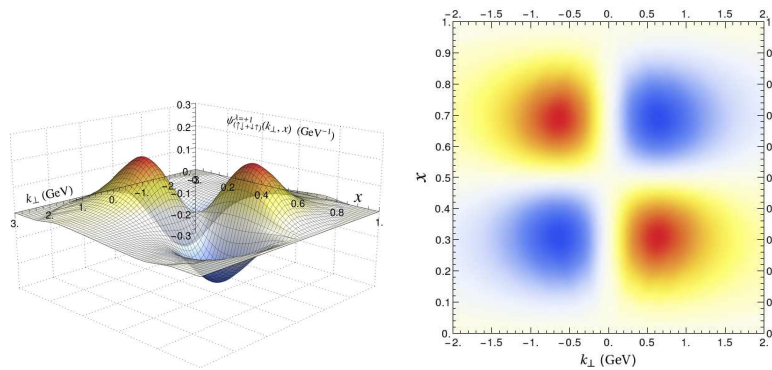

(d)  $\psi_{\uparrow\downarrow\downarrow\uparrow}^{\lambda=+1}(\vec{k}_{\perp}, x)$

Charmonium: X.  $h_c(1P)$



$h_c(1P)$  continued

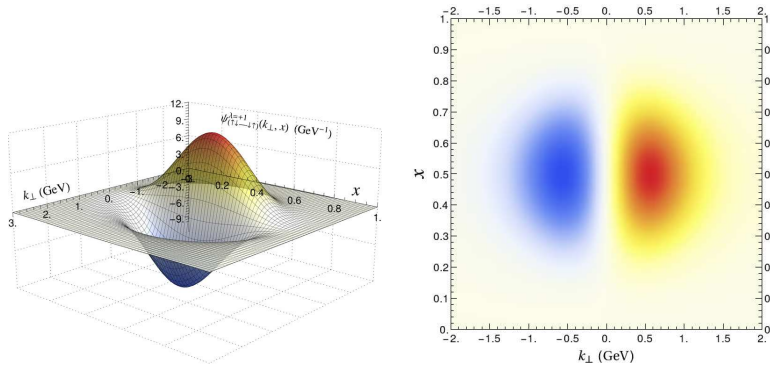

(e)  $\psi_{\uparrow\downarrow}^{\lambda=+1}(\vec{k}_{\perp}, x)$

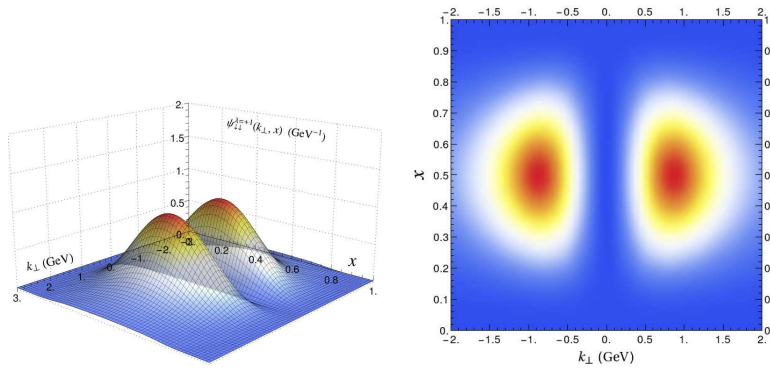

(f)  $\psi_{\uparrow\downarrow}^{\lambda=0}(\vec{k}_{\perp}, x)$

Charmonium: X.  $h_c(1P)$
